# Supplementary material for: The Fundamental Principles of Reproducibility
Source: arXiv:2011.10098 source file (2021-02-22)
Supplement: Supplementary file 1 [file appendix_a.tex]

\section{Appendix A: A Detailed Look at Definitions}
\label{sec:appendic_a}
Here follows the interpretation of the different definitions that is summarized in table~\ref{tab:survey}.

\textbf{Claerbout and Karrenbach \cite{claerbout1992}:} presents a system for making computational research reproducible and Schwab et al. \cite{Schwab_2000} present an evolution of the same system. 
In their work they provide a concrete definition of reproducibility that is the ability to recalculate a figure from all its data, parameters and programs.
Their systems provide a button with each figure in the electronic document that enables the figure to be reproduced using the third party's computer. 
This means compiling and executing all code that implements the experiment on the provided data to produce all immediate and final results.
They argue that written documents are poor at describing the experiment and that the the code the implements the experiments should be shared as well, but the figures with the reproducibility buttons are provided in the electronic document where some description of the experiment is given. 
%Someone else should be able to -> distribution is important
Code generates figures, which means that the analysis should be the same. 
Interpretation is not stated should be the same, although it can be reviewed by independent investigators as all figures are provided. 
Hardware is not explicitly specified, but as third parties should be able to generate figures themselves on their own hardware given code and data, hardware is assumed to be different. 

%implicit at interpretation da blir det samme, men interpretation er ikke spesifisert
%Hardware ikke spesifisert 

\textbf{Buckheit and Donoho \cite{buckheitdonoho95}:} describe WaveLab, which is a library of Matlab that makes available all the code used for produce figures similar to what is presented by Claerbout and Karrenbach \cite{claerbout1992}. 
However, WaveLab is not integrated into the electronic document, but is provided separately. 
The idea is to provide the full environment for which the figures were calculated, but the ancillary software, such as Matlab and the operating systems, is not provided as part of this solution, nor is the hardware, so both are considered to be different.. 
The version of the ancillary software is not automatically documented nor tracked.
The difference between the solutions proposed by Claerbout and Karranbach \cite{claerbout1992} and the one proposed by Buckheit and Donoho \cite{buckheitdonoho95} is therefore a subtle one. 
The solution presented by the latter provides the wavelet libraries used to analyse the data and does not support custom code.
Hence figures and thus analyses can be recreated, but it is up to the independent investigators to interpret the analyses.
%Ancillary software not supported, hence all feature same as Claerbout and Karrenbach.

\textbf{Peng et al. \cite{Peng_2006}:} presents their work on reproducible epidemiologic research. 
They define replication as confirming scientific evidence by multiple independent investigators using independent data, analytical methods, laboratories, and instruments.
Hence, interpretation is interpreted to be the same. 
Independent in their definition is interpreted as \emph{different} and not similar. 
The independent team is not required to use the same experiment design.
Whether all are one of these variables (data, analytical methods etc.) should be different at the same time is not specified.  
%Diff labs = diff ASW, HW
%PRoduce diff results and diff analytical methods 
%interpretation not mentioned
Reproducibility is defined as independent investigators subjecting the original data to their own analyses and interpretations.
Hence, method implementation, ancillary software, hardware, data and outcome are the same, but the analysis and the interpretations are different. 
Hence, replication is defined as being a more general term than reproducibility. 

%%% Replicability is not Reproducibility
\textbf{Drummond\cite{drummond_2009}:} distinguish between reproducibility and replicability and argues that replicability is not worth having. 
Drummond does not clearly specify what exactly is meant by reproducibility and replicability, but states that "Reproducibility requires changes; replicability avoids them."
Furthermore, he states some authors "believe that there should be no difference between one experiment and its reproduction", but he later equates this with "having access to the full code". 
No difference between an experiment and its reproduction indicates that code, hardware and data should be the same and not only code. 
As he refers to third parties having access to full code, I interpret it in that sense and not the very narrow sense of having access to everything including the lab. 
Data is not mentioned specifically, but sharing research artifacts is and the references cited mentions data specifically so it is interpreted as the data should be the same as well.
Replicability means that original research team makes the research artifacts available, not that the results should be the same. 
%Replicability:  different team, same method, implementation, data, analyses as it is code, in my fig of cs. (opptatt av research artifacts.) Others not mentioned => -1 
Reproducibility is to introduce more differences according to Drummond. 
The more differences that are introduced, the stronger the power of the reproducing experiment.  
Experiments on the speed of light is used as an example; the claim is the same for both experiments, but the second experiment proving the claim is completely different from the first.
In this analysis, reproducibility is being interpreted as everything being different but the claim. 
However, Drummond points out that there might be a wide range of differences.  
According to Drummond's analysis, reproducibility is the more general term.
Both are about proving claims, and thus the interpretation should be the same as well. 
%Everything different except for theory and hypothesis

% Shall we really do it again? The powerful concept of replication is neglected in the social sciences
%The term direct replication, which is also used by the Open Science Collaboration \cite{Open_2015} as mentioned above, comes from Schmidt \cite{Schmidt_2009}. 
\textbf{Schmidt \cite{Schmidt_2009}:} distinguishes between two fundamental levels of replication: 1) the narrow bounded notion of replication that is a repetition of experimental procedure termed \emph{direct replication}, and 2) a wider notion of replication that is a test of a hypothesis or a result of earlier research with different methods termed \emph{conceptual replication}. 
Repetition of procedure indicates same method and same implementation, and everything else being different for direct replication. 
Everything but scientific and hypothesis are considered to be different for conceptual replication. 
Schmidt further classifies both direct and conceptual replication into several subclasses.
The subclasses are not considered in the survey. 
While direct replication produce facts, conceptual replication may produce understanding, as direct replication is to redo an experiment with some variations and conceptual replication is to device a new experiment to test a hypothesis and to develop the theories about the world.
Schmidt also introduce the term \emph{confirmatory power}.
Redoing the exact same experiment has no confirmatory power. 
A replication experiment should have both sameness and difference. 
The main function of a replication is to verify a fact or piece of knowledge, but it also have more specific functions, such as 1) control for sampling error, 2) control for artifacts, 3) control for fraud, 4) generalize results for a larger or different population and 5) verify the hypothesis of the earlier experiment. 
Confirmatory power indicates that the interpretations must be the same. 

%Theory => Many claims (general theory of relativity) 
%Hva er en teori i AI? HVor var det jeg leste om dette? Problem solving ethods?
%Noe som forklarer noe
%Hvordan 

%%%%%%%%%%%%%%%%%%%%%%%%%%%%%%%%%%%%%%%%%%%%%%%
%BOOK: STAT AND CHEMOMETRICS FOR ANALYTICAL CHEM.  
\textbf{Miller \cite{Miller_2010}:} distinguishes between repeatability and reproducibilty.
Repeatability is  when the same team repeats an same experiment in the same lab.
Hence, all variables are the same. 
Reproducibility is the when another team performs the same experiment in a different lab. 
It can be expressed in the following equation:
\begin{equation}
\label{eq:reproducibility_standard_deviation}
    S_R^2= S_r^2 + S_L^2,
\end{equation}
where $S_R$ is the reproducibility standard deviation, $S_r$ is the repeatability standard deviation and $S_L$ is the intra-variability between the labs/teams when measuring.
Reproducibility refers to errors in measurements arising in different laboratories and equipment, but using the same analytical methods.
So, this is interpreted that the same implementation is used in a different lab (different hardware and ancillary software) with different data, which will produce different outcome. However, the analysis (analytical methods) is the same. 
Whether the experiments should support the same claims is not mentioned. 
This definition is similar to the one used by Currie and Svehla \cite{Currie_1994} who specify the repeatibility as "the closeness of agreement between independent results obtained with the same method on identical test materials under the same conditions (same operator, same apparatus, same laboratory and after a short time interval)".
Reproducibility is defined as "the closeness of agreement between independent results obtained with the same method on identical test materials but under different conditions (different operator, different apparatus, different laboratory and/or after intervals of time)".
A complete statement of reproducibility requires specification of the experimental conditions which differ. 
Currie and Svehla do not require the same analytical methods and are as such less restrictive. 
%Repeatibility = exact same
%Reproducibility same research artifacts. 
%Anc sw + hw = dif lab, produces own results which are different, data not specified, could be the same in ml but in simulation would be diff. Data reseach artificat = same. 
%Interpretation not mentioned

%%% Reproducible research in computational science
\textbf{Peng \cite{peng_2011}:} analyses reproducibility through the lens of computational sciences, and he introduces the reproducibility spectrum that goes from not reproducible to gold standard.
Papers released without code or data are not reproducible, and the gold standard is full replication.
The reproducibility spectrum has three regions, where the lower end of the spectrum are publications with code, the next region is the papers with code and data and last region is papers with linked and executable code and data. 
According to Peng, reproducibility is related to whether code and data is shared. 
He does not explicitly state or refer to a definition of what exactly is meant by replication.
Also, a paper with code is lower on the spectrum than a paper with code and data. 
The reproducibility spectrum does not cover the situation in which a paper is published with data but no code.
The reproducibility spectrum as proposed to Peng seems to have different characteristics than the electromagnetic spectrum, which has only one dimension namely the wavelength of electromagnetic waves. 
The reproducibility spectrum as proposed is a combination of more variables, both code and data and whether they are linked or not.
The spectrum indicates that a paper without code and data is on the other side of the spectrum from full replication.
This could be interpreted as it is not possible to make a full replication of a published paper, but this is counter-intuitive and is probably not what was intended.
For publication only, methods are interpreted to be the same, but everything else has to be different. 
The hardware and ancillary software do not have to be the same for full replication, so it is interpreted as being different. 
Everything else is considered to be the same, except for interpretation, which is not mentioned. 
Analysis is considered to be the same as it is typically done in code and the code is shared. 
Replication . 

%Also, it is not clear how reproducibility and replicability relate to a paper where no code and data are shared.
%Most papers do not share code and data, but as long as the claims in the papers represent knowledge, they can still be corroborated. 
%The reproducibility spectrum does not capture the fact that hardware and ancillary software, such as operating systems and linked libraries, affect results. 

%%% Trust Your Science? Open Your Data and Code, Stodden 2011
\textbf{Stodden \cite{stodden2011trust}:} also defines repeatability, reproducibility and replicability from the perspective of computational sciences.
According to Stodden, replication is the regeneration of published results from author-provided code and data while reproducibility is a more general term. 
So, interpretation is interpreted as being the same. 
It implies both replication and the regeneration of findings with at least some independence from the code and/or data associated with the original publication. 
This means that some parts must be different, but not necessarily all at the same time. 
Her definition of replication is similar to what Peng calls full replication and reproducibility is similar to direct replication as used by OSF in that changing data represent some independence from the data associated with the original publication. 
Reproducibility could also mean changing the code, but keeping the data. 
Repeatability is mentioned as being more typically used as a term of art referring to the sensitivity of results when underlying measurements are retaken, which relates to the data used in the experiment.
Stodden states that replicability is needed, in part, to resolve differences in outcomes that arise from reproduced computational results, regardless of whether the experiments have been repeated.
%Reproducibility: regeneration of findings -> hypothese? by introducing some independence
%Replication: regeneration of published results from code and data, 

%%% JCGM 2012 MEASUREMENT THEORY %%%
\textbf{Joint Committee for Guides in Metrology \cite{JCGM_2012}:} defines the International Vocabulary of Metrology and the corresponding standard ISO 5725-2 define the  
\begin{enumerate}
    \item \emph{repeatability condition of a measurement (§2.21):}
    a set of conditions that includes the same measurement procedure, same operators, same measuring system, same operating conditions and same location, and replicate measurements on the same or similar objects over a short period of time. That is: same operators, same operating conditions. 
    \item\emph{and as reproducibility condition of a measurement (§2.23):}
    condition of measurement, out of a set of conditions that includes different locations, operators, measuring systems, and replicate measurements on the same or similar objects.
\end{enumerate}
Measurement is interpreted as the same as data for a machine learning system. 
Repeatability and reproducibility conditions are about closeness in measurement precision, which is interpreted as similar outcome.
This allows for drawing the same conclusions, but this is not mentioned. 

%Repeatability => Data = measurements, same, resylts will be similar
%Reproducibility=> different
%Note: The different measuring systems may use different measurement procedures.
%Note: A specification should give the conditions changed and unchanged, to the extent practical.

%%%%%%%%%%%%
\textbf{Crook et al. \cite{Crook_2013}:} describes reproducing results independently in relation to simulators. 
Simulators do not require data, so the authors does not relate their definitions to data. 
The authors distinguish between three different types of replication and reproducibility: 

\begin{description}
\item\emph{Internal replicability:}
The original author or someone in their group can re-create the results in a publication, essentially by rerunning the simulation software. 
For complete replicability within a group by someone other than the original author, especially if simulations are performed months or years later, the author must use proper bookkeeping of simulation details using version control and electronic lab journals.

\item \emph{External replicability:}
A reader is able to re-create the results of a publication using the same tools as the original author. 
As with internal replicability, all implicit knowledge about the simulation details must be entered into a permanent record and shared by the author. 
This approach also relies on code sharing, and readers should be aware that external replicability may be sensitive to the use of different hardware, operating systems, compilers, and libraries.
Analysis is considered the same, as it could be implemented in code. 
Same results is interpreted as same outcome. 

\item \emph{Cross-replicability:} 
The use of “cross” here refers to simulating the same model with different software. This may be achieved by re-implementing a model using a different simulation platform or programming language based on the original code, or by executing a model described in a simulator-independent format on different simulation platforms. 
So, method is interpreted as similar. 
It is not stated that the same result or interpretation is required. 

\item \emph{Reproducibility:} 
Bob reads Alice’s paper, takes note of all model properties, and then implements the model himself using a simulator of his choice. 
This is interpreted as complete reimplementation of method. 
\end{description}
Cross-replicability is independent researchers having access to the specific method that is implemented by the original authors and implementing the same method using a different programming language. 
The method could be described accurately in text or by pseudo code. 
The authors mentioning having access to the code, but implementing it in a different language. 
The above notion is my interpretation. 

%%%% Recomputation Gent & Kotthoff
\textbf{Gent and Kotthoff \cite{gent2013recomputation, gent2014recomputation}:}
present their work with recomputation.org and their effort in simplifying  recomputations - that is to re-execute an computational experiment in the same environment using virtual machines containing the complete experiments. 
In this way the whole environment could be saved and used for executing the exact same experiment in the future.
The goal is that research should be the exact replication of a previous experiment. 
A commitment should be that anyone should be able to compute the experiment 20 years into the future after its publication.
The only thing that might be different is the hardware, although they mentioning emulating the hardware so that the recomputation will be as similar as possible.
They also discuss the notion that the results might differ because of difference in hardware, floating point additions not being associative and differences in temperature.
Results here is interpreted as outcome and that it can be different.
They do not rerquire that the results, that is the conclusions that can be drawn from the experiments to be the same. 

%%% Registered Reports - A Method to Increase the Credibility of Published Results
%%% Estimating the reproducibility of psychological science
\textbf{Nosek and Lakens \cite{Nosek_2014}:} describe a direct replication as "the attempt to duplicate the conditions and procedure that existing theory and evidence anticipate as necessary for obtaining the effect".
The same definition of the term is used in several research articles by the Open Science Collaboration (OSF). 
In a study where OSF seeks to estimate the reproducibility of psychological science \cite{Open_2015}, direct replication is related to reproducibility. 
They state that "direct replication is the attempt to recreate the conditions believed sufficient for obtaining a previously observed finding and is the means of establishing reproducibility of a finding with new data."
Their usage of the term replication seems to indicate that replication is \emph{to follow the same procedures} that were reported in the original experiment as far as possible while reproducibility is establishing the validity of the reported findings with new data.
Same procedure for replication indicates that the method and implementation is the same and that and that ancillary software, hardware, data and outcome are different. 
Establishing validity of reported findings with new data is considered that only data, ancillary software and hardware are different.
Analysis and outcome is not mentioned, but both replication and reproducibility are related to increase the credibility of published results.
Results here is interpreted as being the interpretation. 
%In the end, after replicating 100 experiments, none of the effects were established as true, and hence they reproduced none of the findings. 
%The findings were not falsified either, so the replication studies were indecisive. 
%The notion of direct reproducibility being related to duplicate conditions and procedure used by OSF could be interpreted to keep software and hardware as similar as possible while changing the data in the computational sense. 
%This view of replication is similar to the lowest region of the reproducibility spectrum as proposed by Peng \cite{peng_2011}.
% MÅ gå ordentlig igjennom denne!

%What does reproducibility mean? Goodman et al. 
\textbf{Goodman et al. \cite{Goodman_2016}:} seek to propose a new set of terminology. 
Instead of giving new meanings to the terms reproducibility, replicability and repeatability, they propose to only use reproducibility, but add descriptors of the underlying construct. 
They define three different terms. 
I quote from the paper: 
\begin{description}
\item \emph{Methods reproducibility:} is meant to capture the original meaning of reproducibility, that is, the ability to implement, as exactly as possible, the experimental and computational procedures, with the same data and tools, to obtain the same results.
\item \emph{Results reproducibility:} refers to what was previously described as “replication,” that is, the production of corroborating results in a new study, having followed the same experimental methods. 
\item \emph{Inferential reproducibility:} is the making of knowledge claims of similar strength from a study replication or reanalysis. 
\end{description}
While methods reproducibility seeks to capture reproducibility as proposed by Claerbout et al. \cite{claerbout1992}, namely running the same same code on the exact same data, results reproducibility is more like reading a paper and doing what is described there, which for computer scientists could be interpreted as writing new code and run it on another but similar data set.
Hence, methods reproducibility is the same as reproducibility described by Claerbout et al \cite{claerbout1992}.
Results reproducibility is interpreted as same method, different implementation, ancillary software, hardware, outcome and analysis, but the interpretation must be the same, except that results should be the same, which is interpreted that also the interpretation must be the same. 
Inferential reproducibility is not so straight forward. 
They have to emphasize that "inferential reproducibility is not identical to results reproducibility or to methods reproducibility".
They describe the term using two examples: 1) scientist drawing the same conclusion from different set of studies and 2) scientist drawing different conclusions from the same original data.
As, the definition is unclear and the examples contradict each other in terms of the terms used in this study the term is not documented in this study. 

\textbf{The  Association for Computing Machinery (ACM) \cite{acm_2018}:} provides a seemingly clear definition of repeatability, replicability and reproducibility for computational experiments along the two dimensions team and experimental setup.
Repeatability is defined as the ability of a  researcher to reliably repeat her
own computation, also described as: \emph{same team, same experimental setup}. 
Replicability is defined as an independent group obtaining the same result using the author’s own artifacts or: \emph{different team, same experimental setup}. 
Finally, reproducibility is that an independent group can obtain the same result using artifacts which they develop completely independently, hence: \emph{different team, different experimental setup}. 
A different team using the artifacts of the owner to replicate, does not really mean a different team. 
In computer science, a different team executing the same experiment means just someone else pressing the button. %Artifacts =Z Code and data, not hw
So a different team in this setting probably means running the same code and data using different hardware and ancillary software. 
It could also mean that the different team compiles the code themselves and therefore introduce more difference.
Different laboratory is probably a better term than different team.
It is not clear though how many of the artifacts should be developed by the other team. 
Is it reproducibility if a script setting up the experiment is developed or must all code be implemented by the other team?
Is it enough to use the same artifacts but data,  or must all code and data be changed out with new code and data?
%It seems that reproducibility in the definition given by ACM is not as clear when looking at it in more details.  
%Repeatibility => everything same, results and analysis are implicit as it is stated that researchers should be able to realiably repeat their own computations
%Replicable => Same artifacts
%Reproducibility

%%% State of the Art: Reproducibility in AI
\textbf{Gundersen and Kjensmo \cite{gundersen_kjensmo_2018}:} restrict their definition of reproducibility to empirical AI research. 
According to them, "reproducibility is the ability of an \emph{independent research team} to produce the same \emph{results} using the same \emph{AI method} based on the \emph{documentation} made by the original research team."
Similarly to the ACM definition of reproducibility, they stress the fact that an independent team must conduct the experiment based on the documentation made available by the original team.
Documentation is divided into three categories: code, data and text (AI method and experiment description). 
What constitutes the same results depends on to which degree the results are reproduced.
The idea is that the more documentation that is released by the original team, the results achieved can be more similar.
Three different degrees of reproducibility are introduced: experiment reproducible, data reproducible and method reproducible. 
For an experiment to be considered experiment reproducible, code, data and text must be shared, while only text and data must be shared for the experiment to be considered data reproducible. 
Only text is shared for experiments that are method reproducible.
The same framework for quantifying reproducibility is used by Isdahl and Gundersen \cite{Isdahl_2019} to survey how well machine learning platforms support reproducibility. 

\textbf{National Academies of Science, Engineering, Medicine \cite{national2019}:} define reproducibility and replication and replication is the more general term in their view. 
Reproducibility is defined to mean computational reproducibility, that is to obtaining consistent computational results using the same input data, computational steps, methods, and code, and conditions of analysis; and replicability to mean obtaining consistent results across studies aimed at answering the same scientific question, each of which has obtained its own data. 
In short, reproducibility involves the original data and code; replicability involves new data collection and similar methods used by previous studies.

%%%%%% Brockett 1965
As shown above, the term reproducibility is used in different ways. 
However, they are all related to corroboration of the scientific endeavour. 
A very different usage is put forward by Brockett and Mesarovi{\'c} \cite{Brockett_1965} who suggest to use the term reproducibility in relation to multivariate systems as studied by automation control engineers where the goal is to achieve certain outputs given some inputs values, some transformation functions and state descriptions. 
They propose reproducibility as being one of the properties that reveal the capabilities and limitations of such systems and that reproducibility is the ability to produce some wanted outputs given some inputs.
Reproducibility of the system is its capability of meeting some stated requirements defined as pairs of input and output. 
They also refer to it as output-controllability.
Their usage of the term is limited to whether some control systems are able to reproduce some results given some enforced limitations. 
This notion of reproducibility is very specific to a certain domain and differ from how the term is used today.
The way reproducibility is used by Brockett and Mesarovi{\'c} could be interpreted as meeting some design criteria when designing functions for multivariate systems that have some specified properties related to which input could produce some given output.
As this understanding of reproducibility differ so much from the other definitions above, I will not include this usage in the discussion and summary of findings.

%because scientists might draw the same conclusions from different sets of studies and data or could draw different conclusions from the same original data, sometimes even if they agree on the analytical results.

%"Research reproducibility and other related concepts can be regarded as ways to operationalize truth."

%Transparency vs corroboration => multiple studies corroborating a given result
%Claerbout => Transparency

%"The probability that a claim is true after an experiment is a function of the strength of the new experimen- tal evidence combined with how likely it was to be true before the experiment."
% Diskutere dette i lys av Popper og falsification? Skal det gjøres en annen plass? Digresjon?

1
